# Supplementary material for: DICE: Automatic Emulation of DMA Input Channels for Dynamic Firmware Analysis
Source: arXiv:2007.01502 source file (2021-01-15)
Supplement: Supplementary file 1 [file appendix.tex]

\appendix
\label{ap:appendix}

\subsection{Firmware Tested in Unit Tests and Fuzz-testing}
\label{ap:FirmwareSource}
In this section, we present details about the firmware used in the evaluation section. 
For each firmware, we provide its name, MCU model, OS/SDK, link to source code, etc. 
We also present size of the firmware that are fuzz-tested, which is measured by the ELF file size. 
Table \ref{table:FirmwareUnitTest} presents the firmware used in the unit test, while \ref{table:FirmwareBenchmark} is for firmware fuzz-tested.
